# Supplementary material for: Augmenting the User-Item Graph with Textual Similarity Models
Source: arXiv:2109.09358 source file (2021-09-20)
Supplement: Supplementary file 1 [file appendix.tex]

\section{Basics of Riemannian Geometry}
\label{sec:appendix-riemmanian}

\smallskip
\noindent
\textbf{Manifold:} a $n$-dimensional manifold \manifold{} is a space that can locally be approximated by \realto{n}. It generalizes the notion of a 2D surface to higher dimensions. More concretely, for each point $x$ on \manifold{}, we can find a \textit{homeomorphism} (continuous bijection with continuous inverse) between a neighbourhood of $x$ and \realto{n}.

\smallskip
\noindent
\textbf{Tangent space:} the \textit{tangent space} $T_x \mathcal{M}$ at a point $x$ on \manifold{} is a $n$-dimensional hyperplane in \realto{n+1} that best approximates \manifold{} around $x$. It is the first order linear approximation.

\smallskip
\noindent
\textbf{Riemannian metric:} A \textit{Riemannian metric} $g = (g_x)_{x \in \mathcal{M}}$ on \manifold{} is a collection of inner-products $g_x: T_x \mathcal{M} \times T_x \mathcal{M} \rightarrow \mathbb{R}$ varying smoothly with $x$ on tangent spaces. Riemannian metrics can be used to measure distances on manifolds

\smallskip
\noindent
\textbf{Riemannian manifold:} is a pair $($\manifold{}$, g)$, where \manifold{} is a smooth manifold and $g = (g_x)_{x \in \mathcal{M}}$ is a Riemannian metric.

\smallskip
\noindent
\textbf{Geodesics:} $\gamma: [0,1] \rightarrow$ \manifold{} are the generalizations of straight lines to Riemannian manifolds, i.e., constant speed curves that are locally distance minimizing. In the Poincar\'e disk model, geodesics are circles that are orthogonal to the boundary of the disc as well as diameters.

\smallskip
\noindent
\textbf{Parallel transport:} defined as $P_{x \rightarrow y}: T_x \mathcal{M} \rightarrow T_y \mathcal{M}$, is a linear isometry between tangent spaces that corresponds to moving tangent vectors along geodesics. It is a generalization of translation to non-Euclidean geometry, and it defines a canonical way to connect tangent spaces.

%%%%%%%%%%%%%%%%%%%%%%%%%%%%%
\section{M\"obius Operations}
\label{app:hyperbolic-ops}

\smallskip
\noindent
\textbf{M\"obius addition:}
The hyperbolic analogous to vector addition in Euclidean space is given by the M\"obius addition \cite{ungar2008gyrovector}. For two points $x, y \in \Hy^n$, it is defined as:
\begin{equation}
\small
x \oplus y = \frac{(1 + 2 \langle x,y \rangle + \|y\|^2)x + (1 - \|x\|^2)y}{1 + 2\langle x,y \rangle + \|x\|^2 \|y\|^2}
\end{equation}

\smallskip
\noindent
\textbf{M\"obius matrix-vector multiplication:}
To apply a linear transformation $M: \mathbb{R}^n \rightarrow \mathbb{R}^m$ over a point $x \in \Hy^n, Mx \ne 0$, the M\"obius matrix-vector multiplication is given by \cite{ganea2018hyperNN}:
\begin{equation}
\small
    M \otimes x = \operatorname{tanh}\left(\frac{\|Mx\|}{\|x\|} \operatorname{tanh}^{-1}(\|x\|)\right) \frac{Mx}{\|Mx\|}
\end{equation}

\smallskip
\noindent
\textbf{M\"obius scalar multiplication:} for $x \in \mathbb{D}^n \backslash \{0\}$ the M\"obius scalar multiplication by $r \in$ \real{} is defined as:
\begin{equation}
    r \otimes x = \operatorname{tanh}(r \operatorname{tanh}^{-1}(\|x\|)) \frac{x}{\|x\|}
\end{equation}
and $r \otimes 0 := 0$. By making use of the $\operatorname{exp}$ and $\operatorname{log}$ maps, this expression is reduced to:
\begin{equation}
    r \otimes x = \operatorname{exp}_{\textbf{0}}(r \operatorname{log}_{\textbf{0}}(x)), \quad \forall r \in \mathbb{R}, x \in \mathbb{D}^n
\end{equation}

\smallskip
\noindent
\textbf{Exponential and logarithmic maps:} The mapping between the tangent space and hyperbolic space is done by the exponential map $\operatorname{exp}_{x}: T_x \mathbb{D}^n \rightarrow \mathbb{D}^n$ and the logarithmic map $\operatorname{log}_{x}: \mathbb{D}^n \rightarrow T_x \mathbb{D}^n$. They are given for $v \in T_x \mathbb{D}^n \backslash \{0\}$ and $y \in \mathbb{D}^n \backslash \{0\}, y \ne x$: 

\begin{equation}
\small
\begin{aligned}
& \operatorname{exp}_x(v) = x \oplus \left(\operatorname{tanh}\left(\frac{\lambda_x \|v\|}{2} \right) \frac{v}{\|v\|} \right) \\
& \operatorname{log}_x(y) = \frac{2}{\lambda_x} \operatorname{tanh}^{-1}(\|-x \oplus y\|) \frac{-x \oplus y}{\|-x \oplus y\|}
\end{aligned}
\end{equation}

These expressions become more appealing when $x = 0$, that is, at the origin of the space. It can be seen that the matrix-vector multiplication formula is derived from $M \otimes y = \operatorname{exp}_{\textbf{0}}(M \operatorname{log}_{\textbf{0}}(y))$. 
The point $y \in \mathbb{D}^n$ is mapped to the tangent space $T_\textbf{0} \mathbb{D}^n$, the linear mapping $M$ is applied in the Euclidean subspace, and finally the result is mapped back into the ball. A similar approach holds for the M\"obius scalar multiplication and the application of pointwise non-linearity functions to elements in the Poincar\'e ball (see \cite{ganea2018hyperNN}, Section~2.4).

\smallskip
\noindent
\textbf{Parallel transport with $\operatorname{exp}$ and $\operatorname{log}$ maps:} By applying the $\operatorname{exp}$ and $\operatorname{log}$ maps the parallel transport in the Poincar\'e ball for a vector $v \in T_\textbf{0} \mathbb{D}^n$ to another tangent space $T_x \mathbb{D}^n$, is given by:
\begin{equation}
    P_{\textbf{0} \rightarrow x}(v) = \operatorname{log}_{x}(x \oplus \operatorname{exp}_{\textbf{0}}(v)) = \frac{\lambda_{\textbf{0}}}{\lambda_x} v
\end{equation}
